# Supplementary material for: Scaling Laws for Function Diversity and Specialization Across Socioeconomic and Biological Complex Systems
Source: arXiv:2208.06487 source file (2026-02-12)
Supplement: Supplementary file 1 [file SI.pdf]

# Supplementary Materials

## 1 Null model for function diversity in top-down organizations: weighted random sample

We construct hypothetical organizations of various sizes that are in the range of sizes seen in the data. We first gather the overall frequency of each function,  $i$ ,  $f_i$ , in three classes of organizations—Federal agencies and the two types of universities. The rank-frequency distributions for the number of individuals in each of the functions are shown in Fig. S1. Panel (A) shows the data for Federal agencies, and panels (B) and (C) show the data for universities. We do not have access to the rank-frequency distribution of Norwegian companies. Rank-frequency distributions show curvature (especially in Panels (A) and (B)) and are not power laws.

To construct a hypothetical organizations of size  $N$ , we randomly sample from all available functions  $N$  times, where the probability of each function,  $i$ , being sampled is  $f_i / \sum_{i=1}^D f_i$ . The sampling is done with replacement. We then count the number of unique functions sampled in each organization to produce the prediction shown on the y-axis of the red curves in Fig. S2.

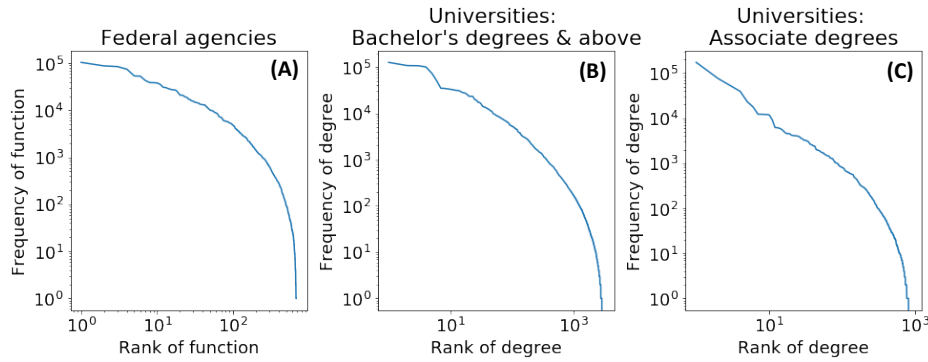

**Figure S1.** The rank-frequency distribution for (A) Occupational functions in federal agencies, (B) University degrees at the Bachelor's level and above, and (C) University degrees at the Associate level.

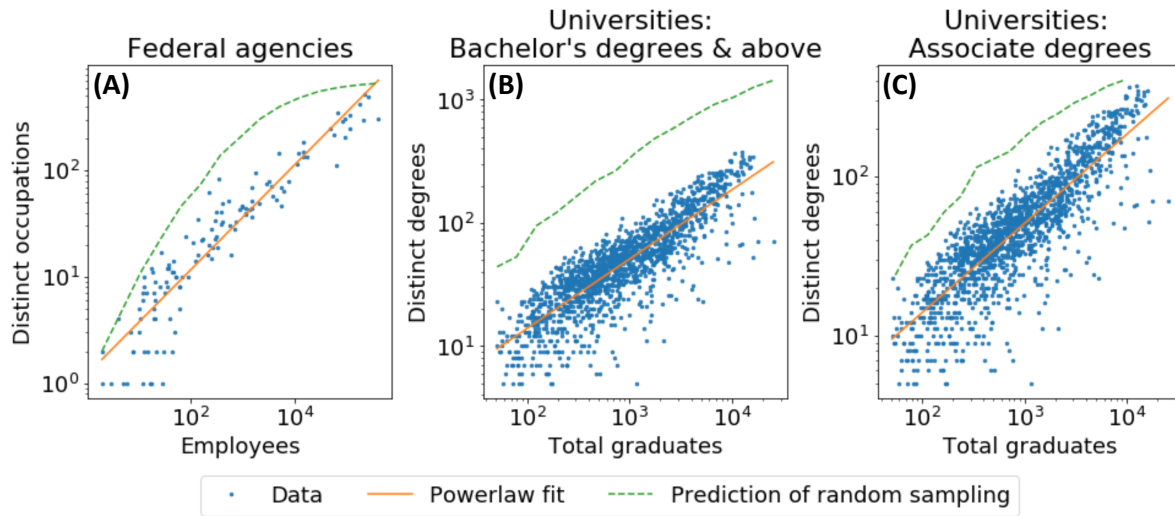

**Figure S2.** Null model sampling and empirical observation: The scaling of distinct functions generated from random sampling of the rank-frequency distribution compared with the data for (A) federal agencies (B) universities offering bachelor's degrees and above, and (C) universities offering associate degrees. Random sampling cannot reproduce the relationship observed in the data.
